# Supplementary material for: Model-Based Reconstruction for Joint Estimation of $T_{1}$, $R_{2}^{*}$ and $B_{0}$ Field Maps Using Single-Shot Inversion-Recovery Multi-Echo Radial FLASH
Source: arXiv:2402.05366 source file (2024-02-08)
Supplement: Supplementary file 1 [file Supporting_Information_File.pdf]

# Supporting Information File

## Model-Based Reconstruction for Joint Estimation of $T_1$, $R_2^*$ and $B_0$ Field Maps Using Single-Shot Inversion-Recovery Multi-Echo Radial FLASH

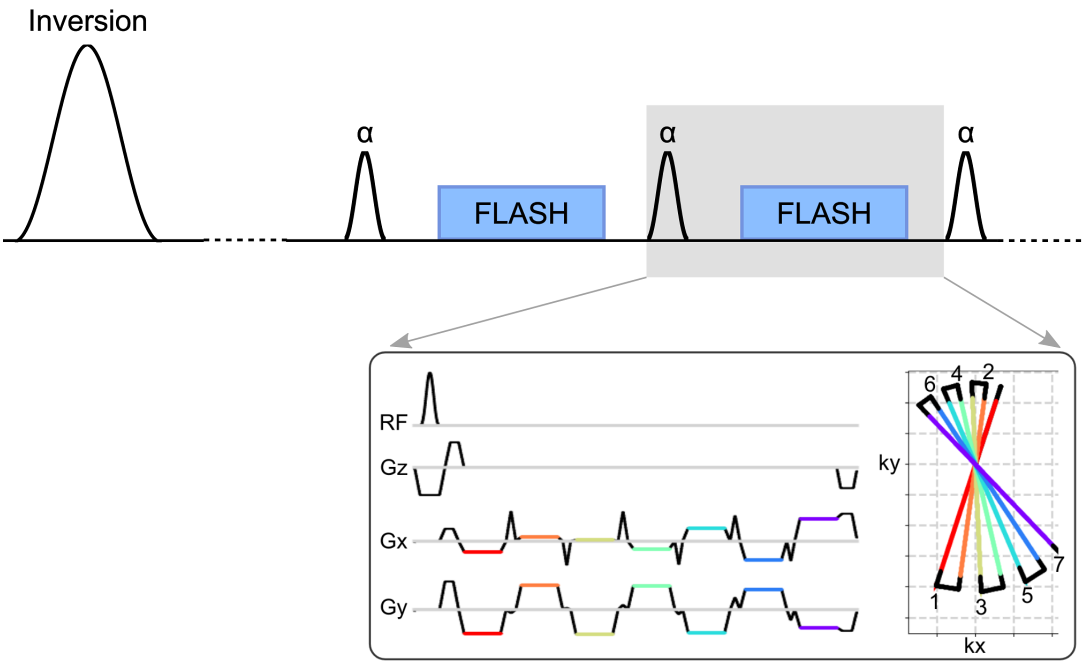


**Supporting Information Figure S1.** Schematic diagram of the single-shot inversion-recovery multi-echo radial FLASH sequence. The distribution of spokes is designed in a way that radial spokes from several TRs (e.g., 9) and all echoes are equally distributed in one $k$-space. Each $k$-space is then rotated by a small golden-angle during inversion recovery. Note that the blip gradients across echoes enable an efficient coverage of $k$-space.

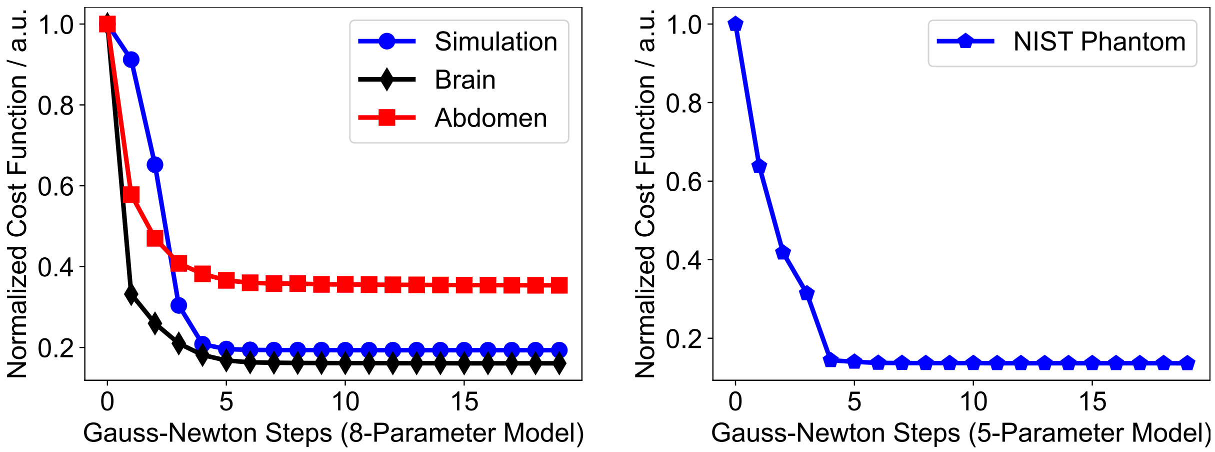


**Supporting Information Figure S2.** Normalized cost function (data fidelity term) as a function of Gauss-Newton steps for different data sets and for both (left) 8-parameter and (right) 5-parameter models.

**Supporting Information Table S1.** Acquisition parameters for IR multi-echo radial FLASH MRI of NIST phantom, human brain, and abdomen.

| | Phantom / Brain | Abdomen |
|---|---|---|
| Field-of-view / $mm^2$ | $220 \times 220$ / $208 \times 208$ | $320 \times 320$ |
| Image matrix | $256 \times 256$ | $200 \times 200$ |
| Resolution | $0.86 \times 0.86$ / $0.81 \times 0.81$ | $1.6 \times 1.6$ |
| Slice thickness / mm | 5 | 6 |
| Repetition time / ms | 15.6 | 10.6 |
| Number of echoes | 7 | 7 |
| Echo times / ms | 2.36/4.26/6.16/8.06/9.96/11.90/13.80 | 1.49/2.61/3.73/4.85/5.97/7.09/8.21 |
| Bandwidth / Hz $pixel^{-1}$ | 810 | 1320 |
| Flip angle / degree | 6 | 6 |
| $N_S$ (No. of TRs) per $k$-space frame | 9 | 9 |
| Total number of excitation | 300 | 360 |
| Total acquisition time / s | 4 | 4 |

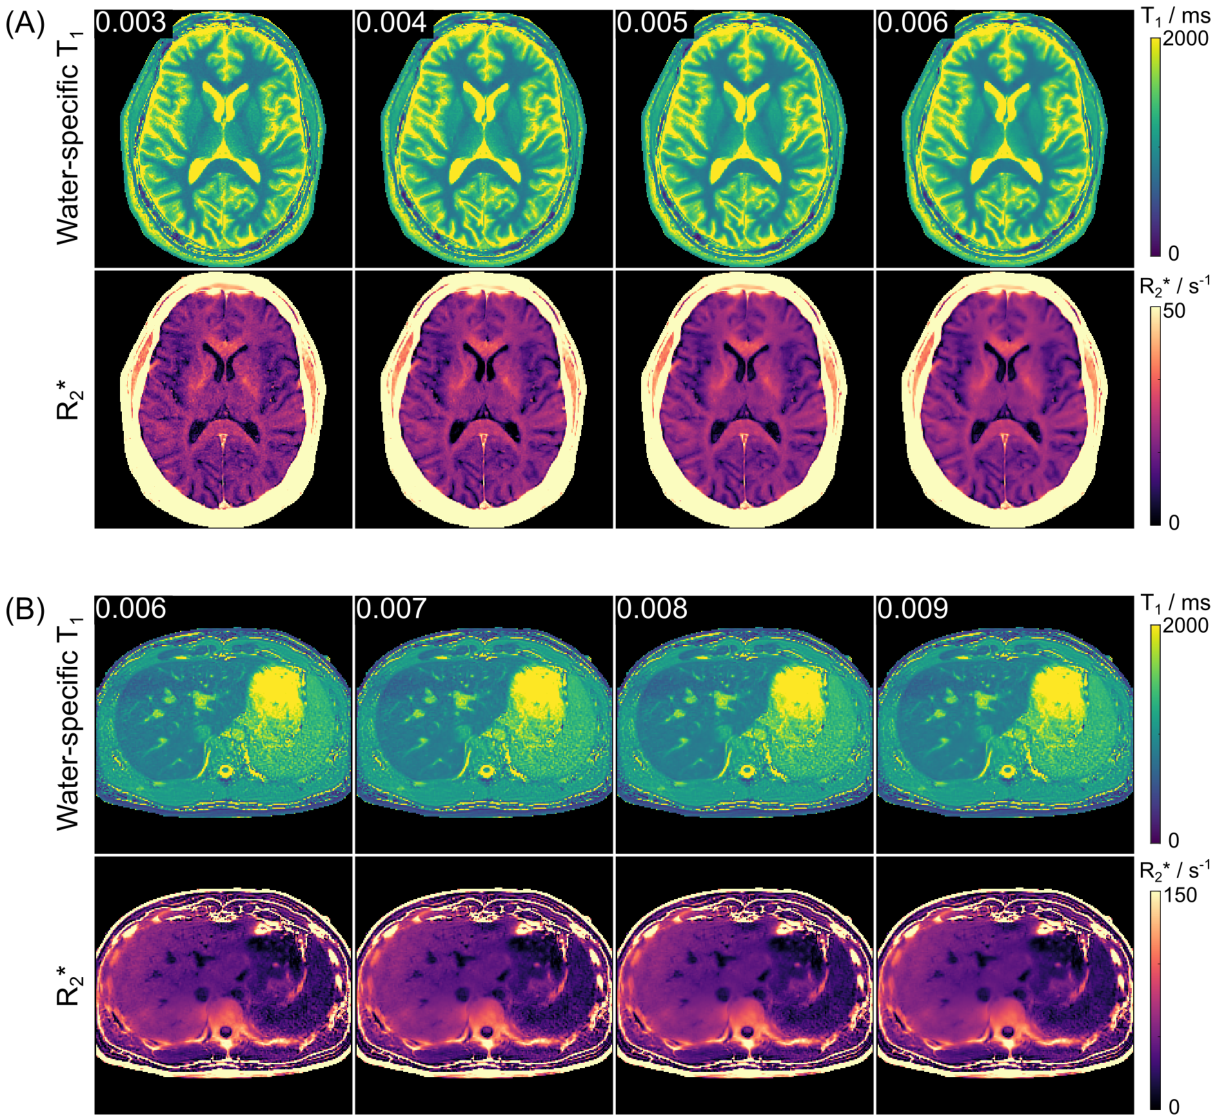


**Supporting Information Figure S3.** (A) Quantitative brain water-specific $T_1$ and $R_2^*$ maps reconstructed with different regularization parameters. (B) The similar comparison for the abdominal study.

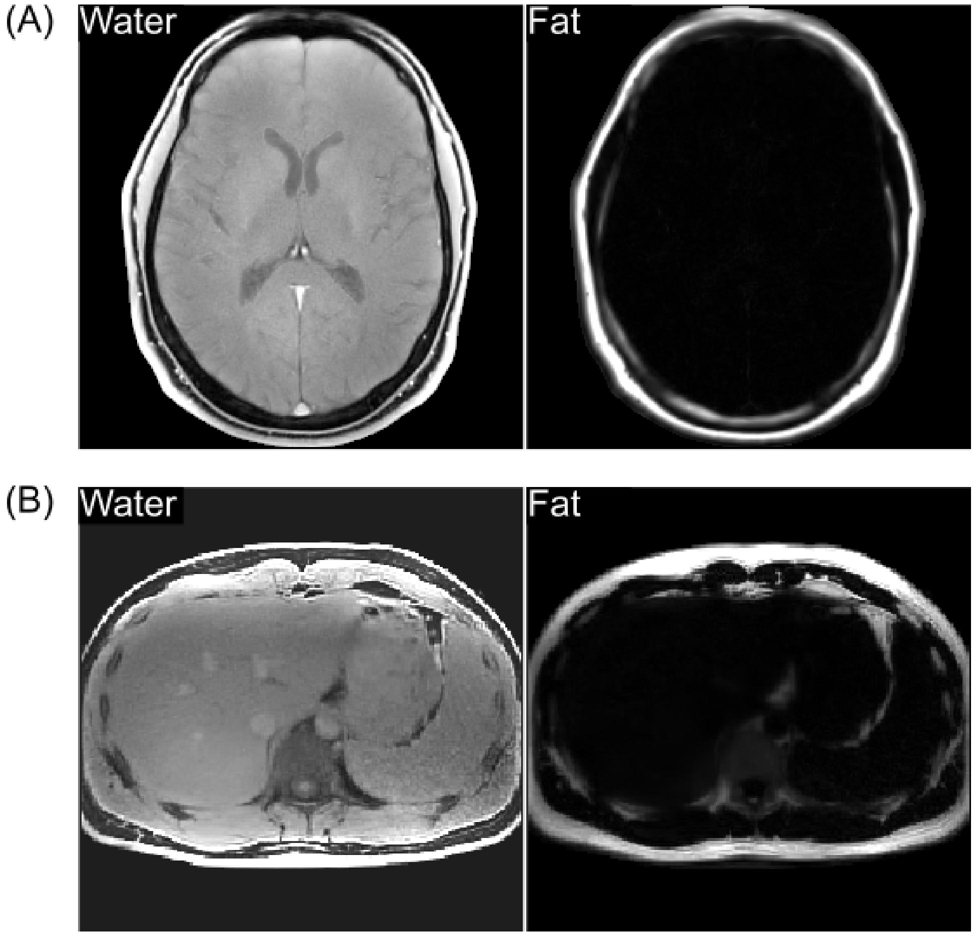


**Supporting Information Figure S4.** Model-based reconstructed water ($W_{ss}$) and fat ($F_{ss}$) images for (A) brain and (B) liver studies.

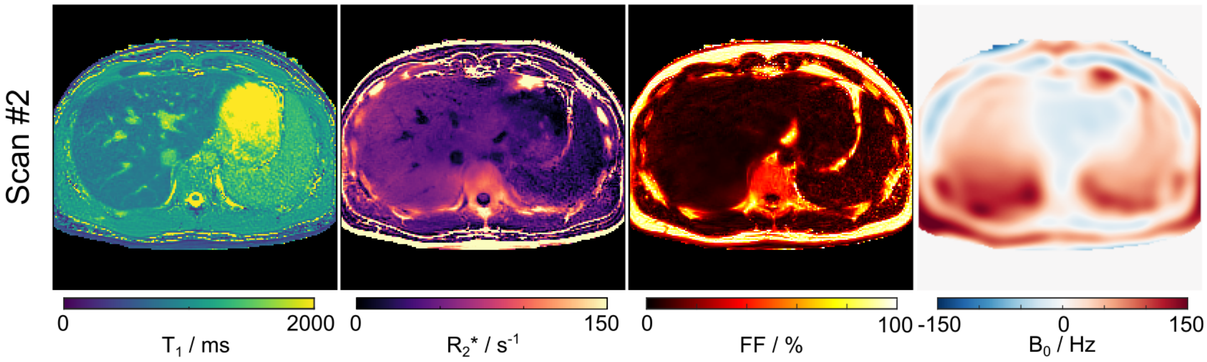


**Supporting Information Figure S5.** Model-based reconstructed liver water-specific $T_1$, $R_2^*$, fat fraction and $B_0$ maps for the second scan.
